# Supplementary material for: Leveraging Key Information Modeling to Improve Less-Data Constrained News Headline Generation via Duality Fine-Tuning
Source: arXiv:2210.04473 source file (2022-10-10)
Supplement: Supplementary file 1 [file Appendix.tex]

\clearpage
\appendix
%\section{Appendix}
\begin{CJK}{UTF8}{gbsn}
\begin{table*}
	\centering\small
	\begin{tabular}{|l|l|l|l|}
		%\hline
		%\multicolumn{4}{|c|}{ggw10k+NE} \\ 
		\hline
		Ground Truth & Normal & Multi-task & Duality \\
		\hline
		\makecell[l]{\colorbox{lightgray}{at\&t业绩}未受\colorbox{lightgray}{verizon推iphone}\\明显影响} & 
		\makecell[l]{\colorbox{lightgray}{at\&t}第一季度新增160万\\非手机联网设备} &
		\makecell[l]{\colorbox{lightgray}{at\&t}第一季度新增160万\\非手机联网设备} & 
		\makecell[l]{\colorbox{lightgray}{at\&t}第一季度\colorbox{lightgray}{业绩}没有受\\到\colorbox{lightgray}{verizon推}出\colorbox{lightgray}{iphone}影响} \\
		\makecell[l]{Translation: \hl{at\&t's performance}\\ is not significantly affected by \\\hl{Verizon's launch of iPhone}} & 
		\makecell[l]{Translation: \hl{at\&t} added \\1.6 million non-mobile \\internet-connected devices\\ in the first quarter} &
		\makecell[l]{Translation: \hl{at\&t} added \\1.6 million non-mobile \\internet-connected devices\\ in the first quarter} & 
		\makecell[l]{Translation: \hl{at\&t}'s first-\\quarter \hl{performance} were not\\ affected by \hl{Verizon's launch}\\\hl{of the iPhone}} \\
		\hline
		\makecell[l]{\colorbox{lightgray}{2gb内存320gb硬盘联想}\\\colorbox{lightgray}{b460el}仅\colorbox{lightgray}{2699元}} & 
		\makecell[l]{gt芯t3500芯\colorbox{lightgray}{联想b460el}\\-tth仅售\colorbox{lightgray}{2699元}} &
		\makecell[l]{i3芯t3500芯\colorbox{lightgray}{联想b460el}\\-tth仅售\colorbox{lightgray}{2699元}} & 
		\makecell[l]{t3500芯\colorbox{lightgray}{320gb硬盘联想}\\\colorbox{lightgray}{b460el}本\colorbox{lightgray}{2699元}} \\
		\makecell[l]{Translation: \hl{2gb memory 320gb} \\\hl{hard disk Lenovo b460el} only \\\hl{2699 yuan}} & 
		\makecell[l]{Translation: gt core t3500\\ core \hl{Lenovo b460el}-tth \\only \hl{2699 yuan}} & 
		\makecell[l]{Translation: i3 core t3500 \\core \hl{Lenovo b460el}-tth \\only \hl{2699 yuan}} & 
		\makecell[l]{Translation: t3500 core \\\hl{320gb hard drive Lenovo}\\\hl{b460el} notebook \hl{2699 yuan}} \\
		\hline
		\makecell[l]{\colorbox{lightgray}{沪指}下挫报收\colorbox{lightgray}{3019.18点}\\\colorbox{lightgray}{创业板全线逆势飘红}} & 
		\makecell[l]{\colorbox{lightgray}{创业板逆势飘红沪指}跌\\1.23\%午后跌幅略有收缩} &
		\makecell[l]{\colorbox{lightgray}{沪}综\colorbox{lightgray}{指}最低跌至3012点\\午后跌幅略有收缩} & 
		\makecell[l]{\colorbox{lightgray}{沪}综\colorbox{lightgray}{指}报收\colorbox{lightgray}{3019.18点}\\\colorbox{lightgray}{创业板全线飘红}} \\
		\makecell[l]{Translation: \hl{Shanghai Composite} \\\hl{Index} fell to close at \hl{3019.18 points}\\ \hl{ChiNext} went \hl{red against the trend}\\\hl{across the board}} & 
		\makecell[l]{Translation: \hl{ChiNext} went \\\hl{red against the trend}, \\\hl{Shanghai index} fell 1.23\%, \\decline slightly contracted\\ in the afternoon} & 
		\makecell[l]{Translation: \hl{Shanghai} \\\hl{Composite Index} fell as low \\as 3012 points in the \\afternoon, decline narrowed\\ slightly} & 
		\makecell[l]{Translation: \hl{Shanghai} \\\hl{Composite Index} closed \\at \hl{3019.18 points}, \hl{ChiNext} \\was \hl{red across the board}} \\
		\hline
		\makecell[l]{\colorbox{lightgray}{报告}称\colorbox{lightgray}{2010年全球无线设备}\\\colorbox{lightgray}{收入}将达\colorbox{lightgray}{2355亿美元}} & 
		\makecell[l]{isuppli预计2011年\colorbox{lightgray}{全球无线}\\\colorbox{lightgray}{设备收入}将达2713亿美元} &
		\makecell[l]{isuppli预计\colorbox{lightgray}{全球无线设备收}\\\colorbox{lightgray}{入}到2011年将达2713亿美元} & 
		\makecell[l]{isuppli称\colorbox{lightgray}{2010年全球无线}\\\colorbox{lightgray}{设备收入}将达\colorbox{lightgray}{2355亿美元}} \\
		\makecell[l]{Translation: \hl{report} says \hl{global} \\\hl{wireless device revenue} to reach\\ \hl{\$235.5 billion} in \hl{2010}} & 
		\makecell[l]{Translation: isuppli expects \\\hl{global wireless equipment}\\ \hl{revenue} to reach \$271.3 \\billion in 2011} & 
		\makecell[l]{Translation: isuppli expects \\\hl{global wireless equipment}\\ \hl{revenue} to reach \$271.3 \\billion by 2011} & 
		\makecell[l]{Translation: isuppli says \\\hl{global wireless equipment}\\ \hl{revenue} will reach \hl{\$235.5}\\ \hl{billion} in \hl{2010}} \\
		\hline
		\makecell[l]{\colorbox{lightgray}{50城100楼盘}发放\colorbox{lightgray}{购房}\\\colorbox{lightgray}{消费券}\colorbox{lightgray}{购房者利益落空}} & 
		\makecell[l]{搜房网\colorbox{lightgray}{购房消费券}发行者\\全国各地媒体曝光} &
		\makecell[l]{房地产行业炒作沸沸扬扬\colorbox{lightgray}{消}\\\colorbox{lightgray}{费券}发行者是全国各地媒体} & 
		\makecell[l]{\colorbox{lightgray}{50}个\colorbox{lightgray}{城}市发券\colorbox{lightgray}{购房}\\\colorbox{lightgray}{消费券}覆盖\colorbox{lightgray}{100}多\colorbox{lightgray}{楼盘}} \\
		\makecell[l]{Translation: \hl{100 real estate} in\\ \hl{50 cities} issued \hl{consumer coupons}\\ \hl{interests of house buyers lost}} & 
		\makecell[l]{Translation: SouFun.com \\issuer of \hl{consumer coupons} \\is exposed by the media \\all over the country} & 
		\makecell[l]{Translation: real estate \\industry hyped, issuer of \\\hl{consumer coupons} is the media\\ from all over the country} & 
		\makecell[l]{Translation: \hl{50 cities} issued\\ \hl{consumer coupons} covering\\ more than \hl{100 real estate}} \\
		\hline
	\end{tabular}
	%\vspace{-2ex}
\caption{\label{casestudy2} Case study on generated headlines with THUCNews dataset. Gray parts are key information. The translation is supported by Google Translate.}
%\vspace{-2ex}
\end{table*}
\end{CJK}

%\footnote{https://translate.google.com/}
